# Supplementary material for: Efficient Diffusion-Driven Corruption Editor for Test-Time Adaptation
Source: arXiv:2403.10911 source file (2024-07-11)
Supplement: Supplementary file 1 [file tab_concat_algs.tex]

\begin{multicols}{2}
\begin{minipage}{0.5\textwidth}
    \begin{algorithm}[H]
     \caption{Decorruptor-DPM/CM Inference}
    \begin{algorithmic}[1]
    \State \textbf{Input:} Text and image guidance scales $\omega_{T}$ and $\omega_{I}$, Given text $c_{T}$ and corrupted image $c_{I}$, Noise schedule $\alpha(t)$, $\sigma(t)$, Decoder $D(\cdot)$ % corrupted image $x_0$ and its latent $z_0$, 
    \State $ts$: Diffusion timesteps (20 for DPM, 4 for CM), $T$: maximum  timesteps (1000) % pre-defined 
    \State $\epsilon_{\theta}$: Pre-trained DPM or CM % pre-defined 
    % \State \textbf{Output:} Generated image $\hat{x}_0$ %and its latent $\hat{z}_0$ 
    \State Sample $\hat{z}_T \sim \mathcal{N}(0;I)$,
    $z \gets \epsilon_\theta(\hat{z}_T, c_{T}, c_{I}, T)$ 
    % \State $\hat{x}_T \gets x_T$
    \For{$t \gets ts \ldots 1$}\hfill $\triangleright$ sequence of timesteps
        \State $\hat{z}_{t} \sim \mathcal{N}(\alpha(t) z; \sigma^2(t) I)$
        \State Eq (7), (9) for DPM, CM $\hfill \triangleright$ multi-modal guidance
        \State $z \gets \epsilon_\theta(\hat{z}_t, c_{T}, c_{I}, t)$ 
        % \State $\hat{x}_{t-1} \sim p_{\theta}(x_{t-1}^g \mid x_t^g)$ \hfill $\triangleright$ unconditional proposal
    \EndFor
    \State $\hat{x}_0 \gets D(z)$ \hfill $\triangleright$ decoding latent to decorrupted image
    \State \textbf{return} $\hat{x}_0$
    \end{algorithmic}
    \label{algorithm1}
    \end{algorithm}
\end{minipage}%
% \hfill
\begin{minipage}{0.5\textwidth}
    \begin{algorithm}[H]
   \caption{Decorruptor-CM Training}
\begin{algorithmic}[1]
\State \textbf{Input:} Given paired dataset $\mathcal{D}^{(p)}$, distance metric $d(\cdot, \cdot)$, pre-trained model parameter $\theta$,learning rate $\eta$, EMA coeff $\mu$, noise schedule $\alpha(t)$, $\sigma(t)$, guidance scale ranges $[w_{I,\min}, w_{I,\max}]$ and $[w_{T,\min}, w_{T,\max}]$, skipping interval $k$, and encoder $E(\cdot)$
\State Encode clean/corrupt data into the latent space: $\mathcal{D}^{(p)}_z = \{(z_{c1}, z_{co}, c) \mid z = E(x), (x_{cl}, x_{co}, c) \in \mathcal{D}^{(p)}\}$
\State $\theta^- \gets \theta$ $\hfill \triangleright$ Initialization
\Repeat
    \State Sample $(z_{cl}, z_{co}, c) \sim \mathcal{D}^{(p)}_z$, $n \sim \mathcal{U}[1, N - k]$
    \State Sample $\epsilon \sim \mathcal{N}(0, I)$, and $w_I$ with $w_T$
    \State $z_{t_{n+k}} \gets \alpha(t_{n+k})z + \sigma(t_{n+k})\epsilon$ 
    \State $z_{t_n} \gets \alpha(t_n)z + \sigma(t_n)\epsilon$
    \State Minimize Eq. (4)
    \State $\theta \gets \theta - \eta \nabla_\theta \mathcal{L}(\theta, \theta^-)$
    \State $\theta^- \gets \text{stopgrad}(\mu \theta^- + (1 - \mu) \theta)$
\Until{convergence}
\end{algorithmic}
\label{algorithm2}
\end{algorithm}
\end{minipage}
\end{multicols}
